# Supplementary material for: Dewetting Fingering Instability in Capillary Suspensions: Role of Particles and Liquid Bridges
Source: arXiv:2412.03306 source file (2025-02-20)
Supplement: Supplementary file 1 [file SI.pdf]

# Supplementary Information for Fingering instability in dewetting capillary nanosuspensions

Lingyue Liu[a,†,*], Mete Abbot[b,†], Philipp Brockmann[b], Ilia V. Roisman[b], Jeanette Hussong[b], Erin Koos[*]

[a] KU Leuven, Department of Chemical Engineering, Celestijnenlaan 200J, 3001 Leuven, Belgium
[b] Technical University of Darmstadt, Institute for Fluid Mechanics and Aerodynamics, Peter-Grünberg-Str. 10, 64287 Darmstadt, Germany
[*] E-mail: lingyue.liu@kuleuven.be, erin.koos@kuleuven.be
[†] These authors contributed to this work equally

## List of Figures

S1 Capillary suspensions without nanoparticles (a) normalized area $A/A_0$ and (b) shrinkage rate over time before cavitation happens per frame (ms). The initial diameters $D_0$ of samples are presented in increasing order from dark blue to dark red. The gray dashed lines are the averaged curves of all the samples shown. The gray areas are the beginning stage where detection fluctuates. . . . . . . . . . . . . 2
S2 The total dendritic skeleton length and overlapped branches with ROI of suspensions with capillary bridges without (a) and with (b) cavitation in their final pattern, dewetted with an acceleration of 50 m/s$^2$. The data are plotted over the normalized radius. . . . . . . . . . . . . . . . . . . . . . . . . . . . . . . . . . . . . . . 3
S3 Capillary suspensions including nanoparticles, with an initial diameter $D_0$ of (a) 27 mm, (b) 27 mm, and (c) 33 mm at different time stamps, dewetted with an acceleration of 50 m/s$^2$. The scale bars are 5 mm. . . . . . . . . . . . . . . . . . . . 3
S4 The residual of capillary suspensions without from the side views, with an initial diameter of (a) 27 mm and (b) 34 mm. The samples are dewetted with an acceleration of 50 m/s$^2$, and the scale bars are 5 mm. . . . . . . . . . . . . . . . . . . . . . . . . 4
S5 Capillary suspensions without nanoparticles lifted with an acceleration of (a) 50 m/s$^2$, (b) 150 m/s$^2$. Capillary suspensions with nanoparticles inside the bridges lifted with an acceleration of (a) 50 m/s$^2$, (b) 150 m/s$^2$. . . . . . . . . . . . . . . . . . . . . . . . 4

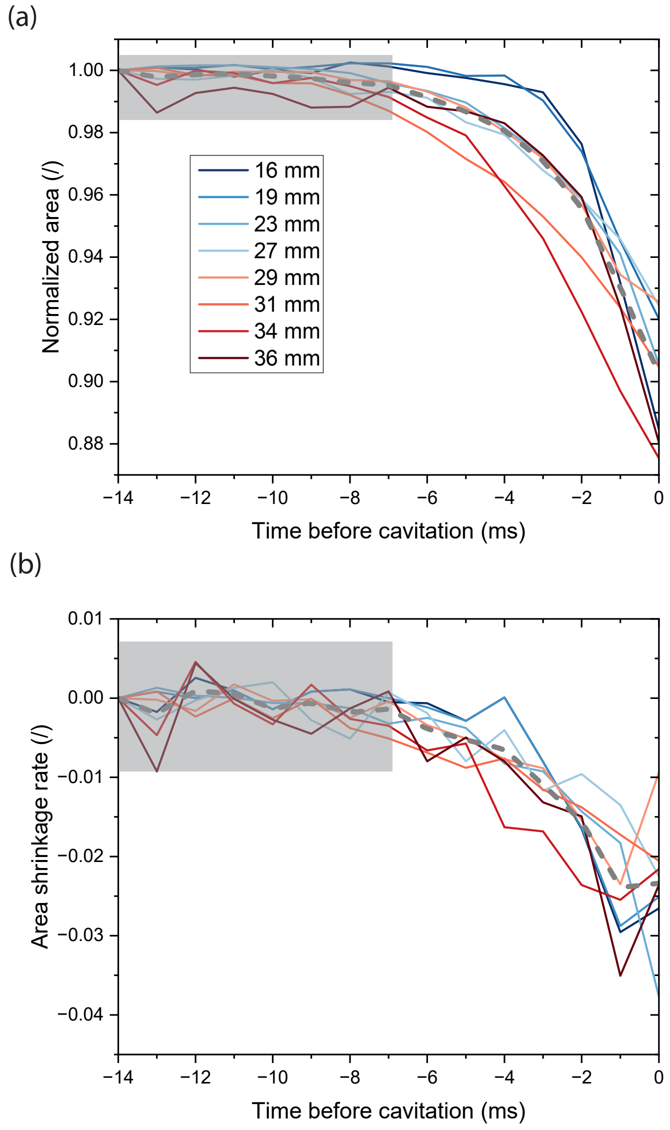


Figure S1: Capillary suspensions without nanoparticles (a) normalized area $A/A_0$ and (b) shrinkage rate over time before cavitation happens per frame (ms). The initial diameters $D_0$ of samples are presented in increasing order from dark blue to dark red. The gray dashed lines are the averaged curves of all the samples shown. The gray areas are the beginning stage where detection fluctuates.

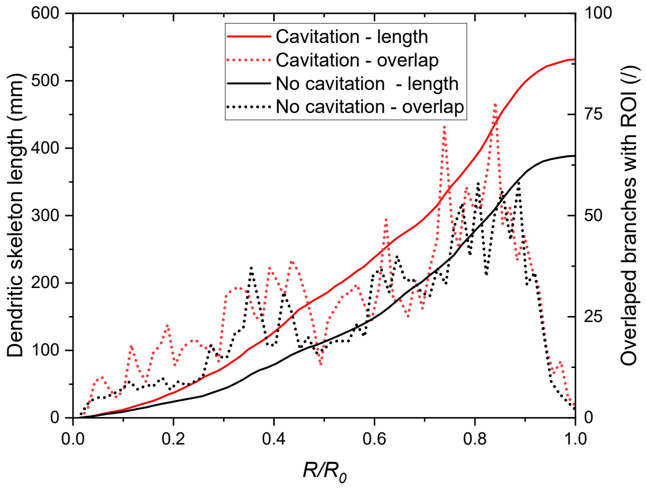


Figure S2: The total dendritic skeleton length and overlapped branches with ROI of suspensions with capillary bridges without (a) and with (b) cavitation in their final pattern, dewetted with an acceleration of 50 $m/s^2$. The data are plotted over the normalized radius.

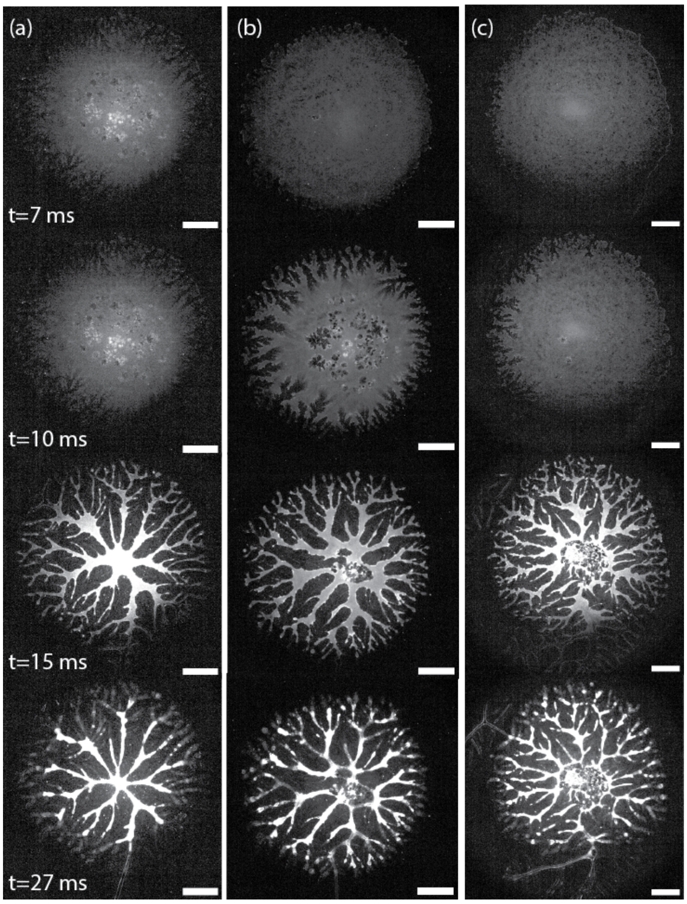


Figure S3: Capillary suspensions including nanoparticles, with an initial diameter $D_0$ of (a) 27 mm, (b) 27 mm, and (c) 33 mm at different time stamps, dewetted with an acceleration of 50 $m/s^2$. The scale bars are 5 mm.

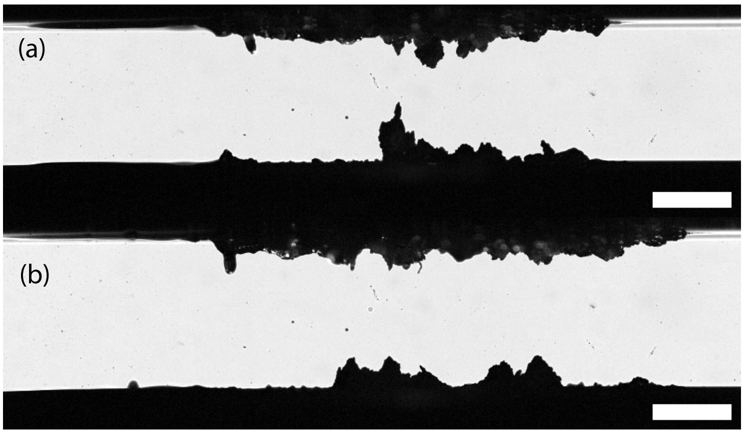


Figure S4: The residual of capillary suspensions without from the side views, with an initial diameter of (a) 27 mm and (b) 34 mm. The samples are dewetted with an acceleration of 50 $m/s^2$, and the scale bars are 5 mm.

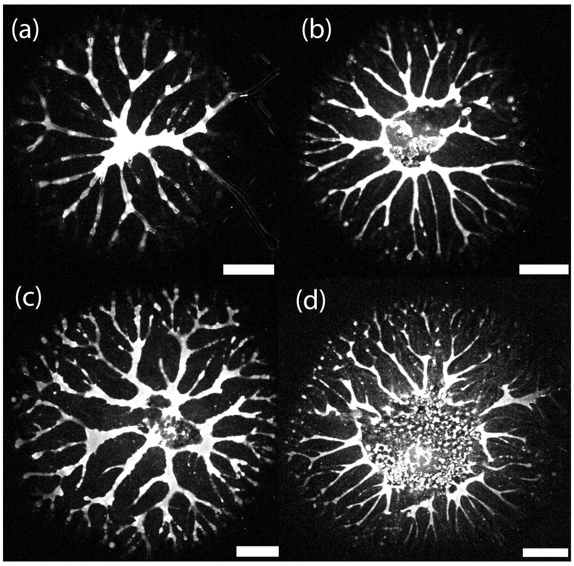


Figure S5: Capillary suspensions without nanoparticles lifted with an acceleration of (a) 50 $m/s^2$, (b) 150 $m/s^2$. Capillary suspensions with nanoparticles inside the bridges lifted with an acceleration of (a) 50 $m/s^2$, (b) 150 $m/s^2$.
